# Supplementary material for: Class-Discriminative CNN Compression
Source: arXiv:2110.10864 source file (2021-10-21)
Supplement: Supplementary file 1 [file model_details.tex]

\section{Pruned Models Details}\label{sec:exp_details}

We show the detailed structures of our pruned VGG-16 and ResNet-50 on ILSVRC-2012 in Table~\ref{tab:VGG-16-Model} and~\ref{tab:ResNet-50-Model}. 
Both pruned models are named as \metric-B in the experimental results section.
On VGG-16, we find that our algorithm prunes more channels in shallow layers, 
which indicates the shallow layers are less sensitive to pruning than the deep ones under the same FLOPs reduction. 
On ResNet-50, our model preserves more channels at the starting blocks of each stage. 
These blocks have stride-2 downsampling connections,
which suggests that preserving information for the resolution reduction process would be crucial to maintain the network's performance.
